# Supplementary material for: Does Mode of Digital Contact Tracing Affect User Willingness to Share Information? A Quantitative Study
Source: arXiv:2210.13399 source file (2022-10-24)
Supplement: Supplementary file 2 [file appendix2.tex]

\newpage
\section{Pairwise Comparison Between Disease Groups}
\label{appx:exploratory}

\begin{figure}[h]
    \centering
    \includegraphics[width=.8\linewidth]{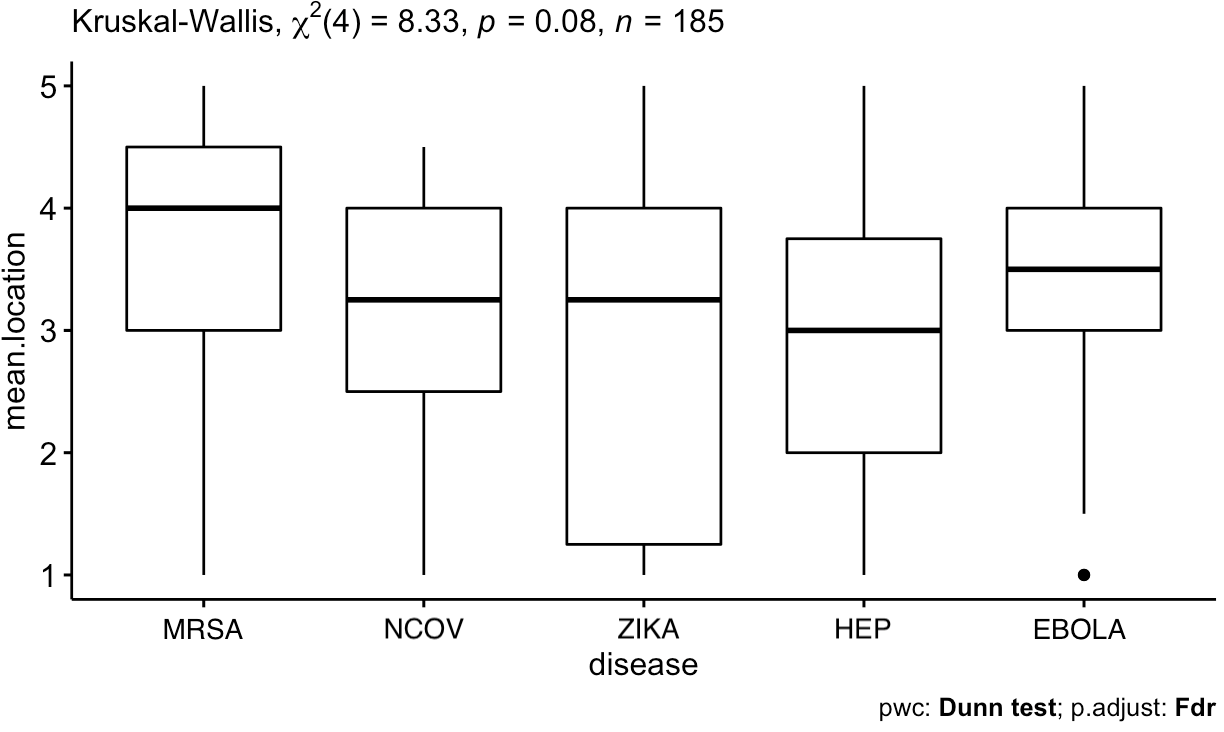}
    \caption{Sharing location data by disease}
    \label{tab:locationPlot}
\end{figure}

\begin{figure}[h]
    \centering
    \includegraphics[width=.85\linewidth]{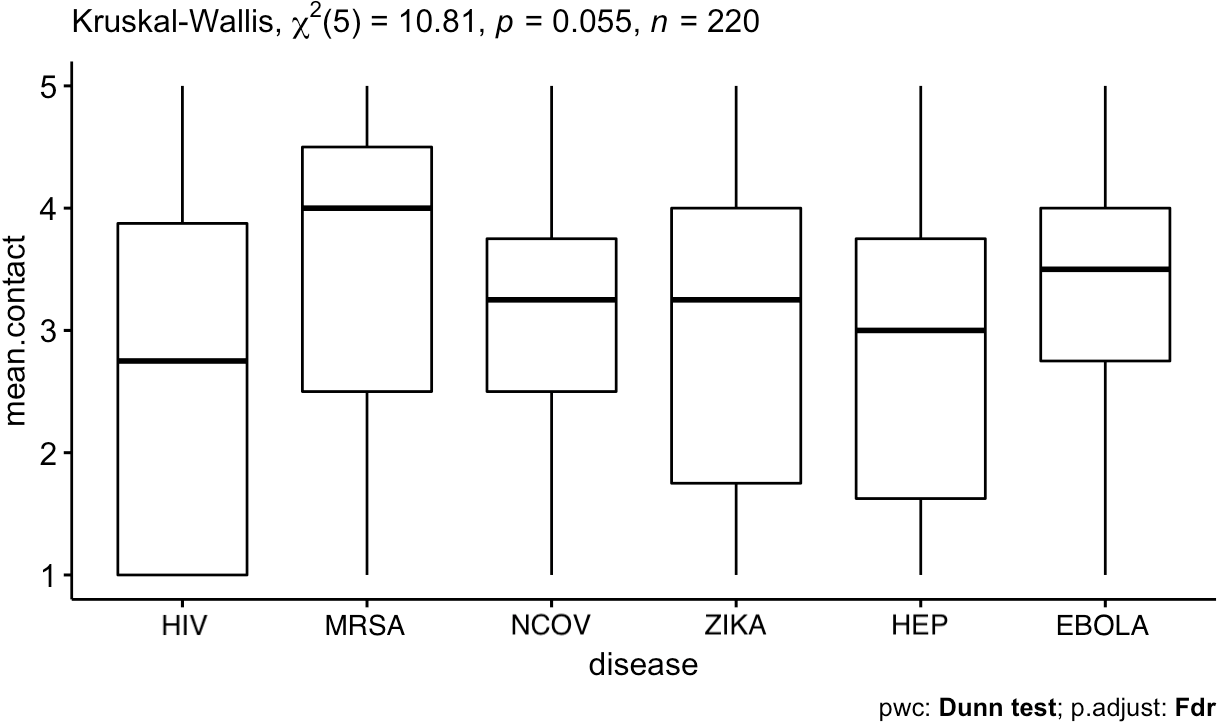}
    \caption{Sharing contact data by disease}
    \label{tab:contactPlot}
\end{figure}

\begin{figure}[h]
    \centering
    \includegraphics[width=.8\linewidth]{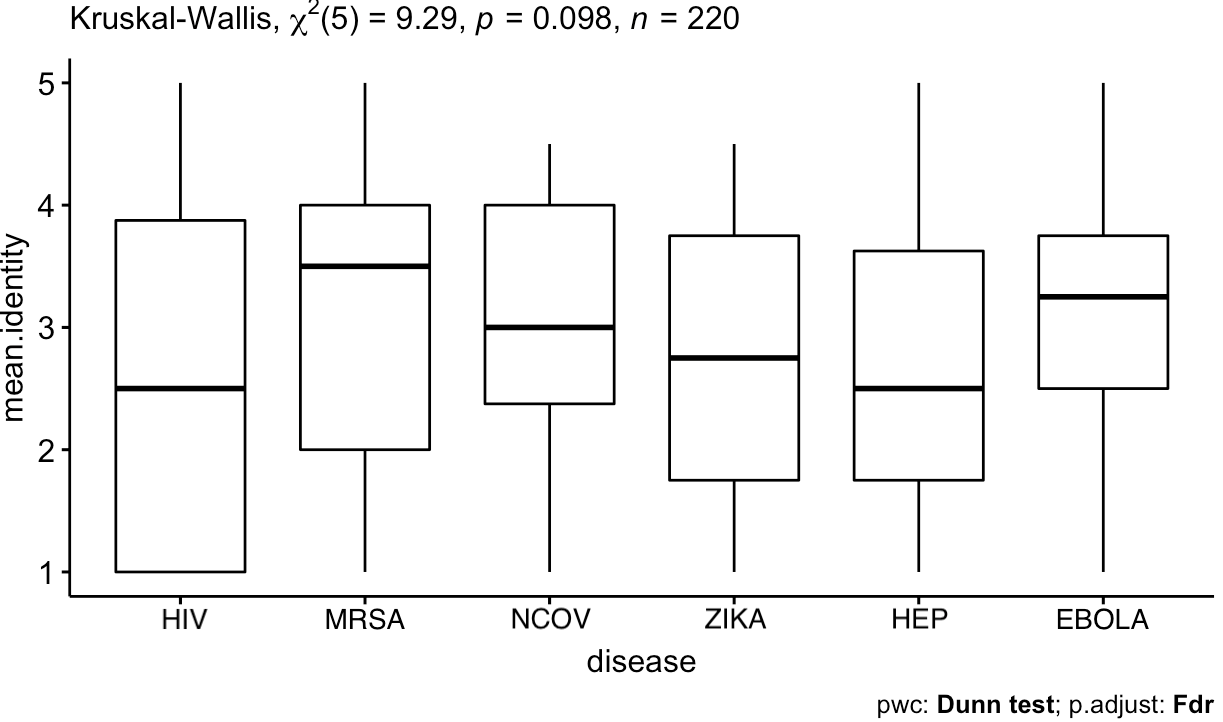}
    \caption{Sharing identity data by disease}
    \label{tab:identityPlot}
\end{figure}

\newpage
\begin{table}[h]
\caption{\revise{Dunn's test p-value summary for location}}
\label{tab:locationDunn}
\resizebox{\linewidth}{!}{
\begin{tabular}{|l|l|l|l|l|l|l|l|}\hline
\toprule
\textbf{Group 1} & \textbf{Group 2} & \textbf{n1} & \textbf{n2} & \textbf{statistic} & \textbf{p} & \textbf{p.adj} & \textbf{Sig} \\
\toprule

MRSA & nCov & 37 & 43 & -2.35 & 0.019 & 0.094 & ns\\
MRSA & Zika & 37 & 37 & -1.95 & 0.051 & 0.171 & ns\\
MRSA & Hep & 37 & 35 & -2.51 & 0.012 & 0.094 & ns\\
MRSA & Ebola & 37 & 33 & -1.19 & 0.234 & 0.469 & ns\\
nCov & Zika & 43 & 37 & 0.329 & 0.742 & 0.777 & ns\\
nCov & Hep & 43 & 35 & -0.284 & 0.777 & 0.777 & ns\\
nCov & Ebola & 43 & 33 & 1.05 & 0.296 & 0.493 & ns\\
Zika & Hep & 37 & 35 & -0.586 & 0.558 & 0.697 & ns\\
Zika & Ebola & 37 & 33 & 0.703 & 0.482 & 0.688 & ns\\
Hep & Ebola & 35 & 33 & 1.26 & 0.206 & 0.469 & ns
\\\hline
\end{tabular}} 
\end{table}

\begin{table}[h]
\caption{\revise{Dunn's test p-value summary for contact}}
\label{tab:contactDunn}
\resizebox{\linewidth}{!}{
\begin{tabular}{|l|l|l|l|l|l|l|l|}\hline
\toprule
\textbf{Group 1} & \textbf{Group 2} & \textbf{n1} & \textbf{n2} & \textbf{statistic} & \textbf{p} & \textbf{p.adj} & \textbf{Sig} \\
\toprule

HIV & MRSA & 35 & 37 & 2.88 & 0.003 & 0.059 & ns\\
HIV & nCov & 35 & 43 & 1.05 & 0.292 & 0.502 & ns\\
HIV & Zika & 35 & 37 & 0.958 & 0.338 & 0.502 & ns\\
HIV & Hep & 35 & 35 & 0.512 & 0.609 & 0.702 & ns\\
HIV & Ebola & 35 & 33 & 1.91 & 0.055 & 0.167 & ns\\
MRSA & nCov & 37 & 43 & -1.96 & 0.049 & 0.167 & ns\\
MRSA & Zika & 37 & 37 & -1.95 & 0.050 & 0.167 & ns\\
MRSA & Hep & 37 & 35 & -2.36 & 0.018 & 0.136 & ns\\
MRSA & Ebola & 37 & 33 & -0.900 & 0.368 & 0.502 & ns\\
nCov & Zika & 43 & 37 & -0.062 & 0.950 & 0.950 & ns\\
nCov & Hep & 43 & 35 & -0.516 & 0.606 & 0.702 & ns\\
nCov & Ebola & 43 & 33 & 0.969 & 0.332 & 0.502 & ns\\
Zika & Hep & 37 & 35 & -0.439 & 0.661 & 0.708 & ns\\
Zika & Ebola & 37 & 33 & 0.996 & 0.319 & 0.502 & ns\\
Hep & Ebola & 35 & 33 & 1.41 & 0.159 & 0.397 & ns
\\\hline
\end{tabular}} 
\end{table}

\begin{table}[h]
\caption{\revise{Dunn's test p-value summary for identity}}
\label{tab:identityDunn}
\resizebox{\linewidth}{!}{
\begin{tabular}{|l|l|l|l|l|l|l|l|}\hline
\toprule
\textbf{Group 1} & \textbf{Group 2} & \textbf{n1} & \textbf{n2} & \textbf{statistic} & \textbf{p} & \textbf{p.adj} & \textbf{Sig} \\
\toprule

HIV & MRSA & 35 & 37 & 2.38 & 0.017 & 0.152 & ns\\
HIV & nCov & 35 & 43 & 1.06 & 0.287 & 0.524 & ns\\
HIV & Zika & 35 & 37 & 0.454 & 0.650 & 0.740 & ns\\
HIV & Hep & 35 & 35 & 0.055 & 0.956 & 0.956 & ns\\
HIV & Ebola & 35 & 33 & 1.73 & 0.083 & 0.282 & ns\\
MRSA & nCov & 37 & 43 & -1.42 & 0.156 & 0.389 & ns\\
MRSA & Zika & 37 & 37 & -1.95 & 0.051 & 0.255 & ns\\
MRSA & Hep & 37 & 35 & -2.32 & 0.020 & 0.152 & ns\\
MRSA & Ebola & 37 & 33 & -0.590 & 0.555 & 0.694 & ns\\
nCov & Zika & 43 & 37 & -0.603 & 0.546 & 0.694 & ns\\
nCov & Hep & 43 & 35 & -1.01 & 0.314 & 0.524 & ns\\
nCov & Ebola & 43 & 33 & 0.766 & 0.444 & 0.666 & ns\\
Zika & Hep & 37 & 35 & -0.398 & 0.691 & 0.740 & ns\\
Zika & Ebola & 37 & 33 & 1.30 & 0.192 & 0.411 & ns\\
Hep & Ebola & 35 & 33 & 1.67 & 0.094 & 0.282 & ns
\\\hline
\end{tabular}} 
\end{table}
